# Supplementary material for: Design of a multifunctional polar metal via first-principles high-throughput structure screening
Source: arXiv:1901.08771 source file (2020-02-05)
Supplement: Supplementary file 1 [file polar-metal-supp.pdf]

**Supplementary Information for:**  
**Design of a new multifunctional polar metal via first-principles**  
**high-throughput structure screening**

Yue-Wen Fang<sup>1,2\*</sup> and Hanghui Chen<sup>2,3†</sup>

<sup>1</sup>*Department of Materials Science and Engineering, Kyoto University, Kyoto, Japan*

<sup>2</sup>*NYU-ECNU Institute of Physics, New York University Shanghai China*

<sup>3</sup>*Department of Physics, New York University, New York 10003, USA*

(Dated: September 19, 2019)

---

\* fyuewen@gmail.com

† hanghui.chen@nyu.edu

## I. LOW-ENERGY STRUCTURES PREDICTED FROM CALYPSO SEARCH

TABLE S1. A list of predicted crystal structures including ten lowest energy states, perovskite anti-polar state with  $Pmma$  symmetry, and post-perovskite anti-polar state with  $Pmmm$  symmetry. ‘—’ represents non-perovskite and non-post-perovskite structures. Post-perovskite structures are explicitly shown. ‘Layered’, ‘Rock-salt’, and ‘Columnar’ refer to different cation orderings of  $A$ -site ordered double perovskite structure (the naming convention follows Ref. [1]).

| Phase    | Cell parameters         | Atom type | Wyckoff site | X      | Y     | Z     | Ordering          | $E$ (meV) |
|----------|-------------------------|-----------|--------------|--------|-------|-------|-------------------|-----------|
| $Pmm2$   | $a = 5.616 \text{ \AA}$ | Ti1       | 2g           | 0.483  | 0.251 | 0.000 | Post-perovskite 0 |           |
|          |                         | Bi1       | 1c           | -0.074 | 0.000 | 0.500 |                   |           |
|          | $b = 3.035 \text{ \AA}$ | Pb1       | 1d           | 0.018  | 0.500 | 0.500 |                   |           |
|          | $c = 7.597 \text{ \AA}$ | O1        | 2h           | 0.264  | 0.216 | 0.500 |                   |           |
|          | $\alpha = 90.000^\circ$ | O2        | 2h           | 0.724  | 0.270 | 0.500 |                   |           |
|          | $\beta = 90.000^\circ$  | O3        | 1a           | 0.575  | 0.000 | 0.000 |                   |           |
|          | $\gamma = 90.000^\circ$ | O4        | 1b           | 0.439  | 0.500 | 0.000 |                   |           |
|          |                         |           |              |        |       |       |                   |           |
| $Pmn2_1$ | $a = 5.520 \text{ \AA}$ | Ti1       | 4b           | 0.056  | 0.742 | 0.749 | Rock-salt         | 93.0      |
|          |                         | Bi1       | 2a           | 0.517  | 0.785 | 0.000 |                   |           |
|          | $b = 5.543 \text{ \AA}$ | Pb1       | 2a           | 0.039  | 0.258 | 0.000 |                   |           |
|          | $c = 7.993 \text{ \AA}$ | O1        | 4b           | 0.279  | 0.463 | 0.736 |                   |           |
|          | $\alpha = 90.000^\circ$ | O2        | 4b           | 0.860  | 0.045 | 0.746 |                   |           |
|          | $\beta = 90.000^\circ$  | O3        | 2a           | 0.099  | 0.750 | 0.000 |                   |           |
|          | $\gamma = 90.000^\circ$ | O4        | 2b           | 0.557  | 0.221 | 0.000 |                   |           |
|          |                         |           |              |        |       |       |                   |           |
| $Pmm2$   | $a = 4.077 \text{ \AA}$ | Ti1       | 2g           | 0.542  | 0.000 | 0.245 | Layered           | 93.2      |
|          |                         | Bi1       | 1d           | 0.129  | 0.500 | 0.500 |                   |           |
|          | $b = 3.919 \text{ \AA}$ | Pb1       | 1c           | 0.079  | 0.500 | 0.000 |                   |           |
|          | $c = 7.887 \text{ \AA}$ | O1        | 2g           | -0.014 | 0.000 | 0.253 |                   |           |
|          | $\alpha = 90.000^\circ$ | O2        | 2h           | 0.457  | 0.500 | 0.259 |                   |           |
|          | $\beta = 90.000^\circ$  | O3        | 1a           | 0.480  | 0.000 | 0.000 |                   |           |
|          | $\gamma = 90.000^\circ$ | O4        | 1b           | 0.441  | 0.000 | 0.500 |                   |           |
|          |                         |           |              |        |       |       |                   |           |

|             |                          |     |    |        |        |        |           |       |
|-------------|--------------------------|-----|----|--------|--------|--------|-----------|-------|
| <i>P1</i>   |                          | Ti1 | 1a | 0.312  | 0.738  | 0.155  | —         | 103.4 |
|             |                          | Ti2 | 1a | 0.425  | 0.835  | 0.381  |           |       |
|             |                          | Ti3 | 1a | 0.621  | 0.175  | 0.768  |           |       |
|             |                          | Ti4 | 1a | 0.719  | 0.710  | -0.033 |           |       |
|             |                          | Bi1 | 1a | 0.014  | 0.244  | 0.538  |           |       |
|             |                          | Bi2 | 1a | 0.044  | 0.768  | 0.617  |           |       |
|             |                          | Pb1 | 1a | 0.221  | 0.216  | -0.030 |           |       |
|             | $a = 3.743 \text{ \AA}$  | Pb2 | 1a | 0.865  | 0.252  | 0.286  |           |       |
|             | $b = 5.943 \text{ \AA}$  | O1  | 1a | 0.136  | 0.189  | 0.797  |           |       |
|             | $c = 13.435 \text{ \AA}$ | O2  | 1a | 0.237  | 0.735  | 0.002  |           |       |
|             | $\alpha = 93.478^\circ$  | O3  | 1a | 0.336  | 0.024  | 0.200  |           |       |
|             | $\beta = 97.928^\circ$   | O4  | 1a | 0.371  | 0.587  | 0.271  |           |       |
|             | $\gamma = 90.068^\circ$  | O5  | 1a | 0.451  | 0.161  | 0.423  |           |       |
|             |                          | O6  | 1a | 0.485  | 0.706  | 0.498  |           |       |
|             |                          | O7  | 1a | 0.563  | 0.314  | 0.649  |           |       |
|             |                          | O8  | 1a | 0.590  | 0.884  | 0.708  |           |       |
|             |                          | O9  | 1a | 0.682  | 0.450  | 0.891  |           |       |
|             |                          | O10 | 1a | 0.694  | -0.009 | -0.085 |           |       |
| <i>I4mm</i> |                          | O11 | 1a | 0.793  | 0.665  | 0.115  | Rock-salt | 109.1 |
|             |                          | O12 | 1a | -0.086 | 0.883  | 0.356  |           |       |
|             | $a = 5.561 \text{ \AA}$  | Ti1 | 4b | 0.000  | 0.500  | 0.216  |           |       |
|             | $b = 5.561 \text{ \AA}$  | Bi1 | 2a | 0.000  | 0.000  | 0.508  |           |       |
|             | $c = 8.161 \text{ \AA}$  | Pb1 | 2a | 0.000  | 0.000  | -0.016 |           |       |
|             | $\alpha = 90.000^\circ$  | O1  | 8c | 0.743  | 0.743  | 0.173  |           |       |
|             | $\beta = 90.000^\circ$   | O2  | 4b | 0.000  | 0.500  | 0.437  |           |       |
|             | $\gamma = 90.000^\circ$  |     |    |        |        |        |           |       |

|              |                          |     |    |       |       |         |           |       |
|--------------|--------------------------|-----|----|-------|-------|---------|-----------|-------|
| $Cm$         | $a = 7.923 \text{ \AA}$  | Ti1 | 4b | 0.465 | 0.257 | 0.0.060 | Columnar  | 120.0 |
|              | $b = 7.875 \text{ \AA}$  | Bi1 | 2a | 0.667 | 0.000 | 0.622   |           |       |
|              | $c = 3.972 \text{ \AA}$  | Pb1 | 2a | 0.201 | 0.000 | 0.577   |           |       |
|              | $\alpha = 90.000^\circ$  | O1  | 4b | 0.224 | 0.285 | 0.036   |           |       |
|              | $\beta = 90.000^\circ$   | O2  | 4b | 0.484 | 0.245 | 0.551   |           |       |
|              | $\gamma = 90.000^\circ$  | O3  | 2a | 0.006 | 0.000 | 0.051   |           |       |
|              |                          | O4  | 2b | 0.460 | 0.000 | 0.031   |           |       |
|              |                          |     |    |       |       |         |           |       |
| $R32$        | $a = 5.475 \text{ \AA}$  | Ti1 | 6c | 0.000 | 0.000 | 0.747   | Rock-salt | 137.3 |
|              | $b = 5.475 \text{ \AA}$  | Bi1 | 3b | 0.000 | 0.000 | 0.500   |           |       |
|              | $c = 5.475 \text{ \AA}$  | Pb1 | 3a | 0.000 | 0.000 | 0.000   |           |       |
|              | $\alpha = 61.727^\circ$  | O1  | 9d | 0.449 | 0.000 | 0.000   |           |       |
|              | $\beta = 61.727^\circ$   | O2  | 9e | 0.573 | 0.000 | 0.500   |           |       |
|              | $\gamma = 61.727^\circ$  |     |    |       |       |         |           |       |
|              |                          |     |    |       |       |         |           |       |
| $P2_12_12$   | $a = 5.494 \text{ \AA}$  | Ti1 | 4c | 0.501 | 0.750 | 0.252   | Rock-salt | 138.3 |
|              | $b = 7.980 \text{ \AA}$  | Bi1 | 2b | 0.000 | 0.500 | 0.233   |           |       |
|              | $c = 5.498 \text{ \AA}$  | Pb1 | 2a | 0.000 | 0.000 | 0.253   |           |       |
|              | $\alpha = 90.000^\circ$  | O1  | 4c | 0.699 | 0.239 | 0.548   |           |       |
|              | $\beta = 90.000^\circ$   | O2  | 4c | 0.704 | 0.759 | -0.048  |           |       |
|              | $\gamma = 90.000^\circ$  | O3  | 2a | 0.000 | 0.000 | 0.749   |           |       |
|              |                          | O4  | 2b | 0.000 | 0.500 | 0.764   |           |       |
|              |                          |     |    |       |       |         |           |       |
| $I\bar{4}2m$ | $a = 5.492 \text{ \AA}$  | Ti1 | 4d | 0.000 | 0.500 | 0.250   | Rock-salt | 139.4 |
|              | $b = 5.492 \text{ \AA}$  | Bi1 | 2b | 0.000 | 0.000 | 0.500   |           |       |
|              | $c = 5.569 \text{ \AA}$  | Pb1 | 2a | 0.000 | 0.000 | 0.000   |           |       |
|              | $\alpha = 119.545^\circ$ | O1  | 8i | 0.201 | 0.201 | 0.260   |           |       |
|              | $\beta = 119.545^\circ$  | O2  | 4c | 0.000 | 0.500 | 0.000   |           |       |
|              | $\gamma = 90.000^\circ$  |     |    |       |       |         |           |       |
|              |                          |     |    |       |       |         |           |       |

|             |                          |     |    |        |         |       |                 |       |
|-------------|--------------------------|-----|----|--------|---------|-------|-----------------|-------|
| <i>Pnnm</i> | $a = 5.4916 \text{ \AA}$ | Ba1 | 2b | 0.000  | 0.000   | 0.500 | Rock-salt       | 135.0 |
|             | $b = 5.4915 \text{ \AA}$ | Pb1 | 2a | 0.000  | 0.000   | 0.000 |                 |       |
|             | $c = 7.9943 \text{ \AA}$ | Ti1 | 4f | 0.000  | 0.500   | 0.750 |                 |       |
|             | $\alpha = 90.000^\circ$  | O1  | 8h | 0.7024 | 0.70239 | 0.761 |                 |       |
|             | $\beta = 90.000^\circ$   | O2  | 2c | 0.000  | 0.500   | 0.000 |                 |       |
|             | $\gamma = 90.000^\circ$  | O3  | 2d | 0.000  | 0.500   | 0.500 |                 |       |
| <i>Pmma</i> | $a = 3.945 \text{ \AA}$  | Ti1 | 4j | 0.500  | 0.492   | 0.378 | Layered         | 158.0 |
|             | $b = 3.951 \text{ \AA}$  | Bi1 | 2e | 0.000  | 0.882   | 0.250 |                 |       |
|             | $c = 15.859 \text{ \AA}$ | Pb1 | 2a | 0.000  | 0.000   | 0.000 |                 |       |
|             | $\alpha = 90.000^\circ$  | O1  | 2d | 0.500  | 0.500   | 0.000 |                 |       |
|             | $\beta = 90.000^\circ$   | O2  | 4j | 0.500  | 0.012   | 0.126 |                 |       |
|             | $\gamma = 90.000^\circ$  | O3  | 4i | 0.000  | 0.531   | 0.131 |                 |       |
|             |                          | O4  | 2f | 0.500  | 0.553   | 0.250 |                 |       |
|             |                          |     |    |        |         |       |                 |       |
| <i>Pmmm</i> | $a = 3.057 \text{ \AA}$  | Bi1 | 1b | 0.500  | 0.000   | 0.000 | Post-perovskite | 218.5 |
|             | $b = 7.637 \text{ \AA}$  | Pb1 | 1f | 0.500  | 0.500   | 0.000 |                 |       |
|             | $c = 5.539 \text{ \AA}$  | Ti1 | 2n | 0.000  | 0.249   | 0.500 |                 |       |
|             | $\alpha = 90.000^\circ$  | O1  | 4v | 0.500  | 0.242   | 0.263 |                 |       |
|             | $\beta = 90.000^\circ$   | O2  | 1c | 0.000  | 0.000   | 0.500 |                 |       |
|             | $\gamma = 90.000^\circ$  | O3  | 1g | 0.000  | 0.500   | 0.500 |                 |       |

In our structure search, we consider all possible cation orderings in perovskite structure, as well as non-perovskite structures such as post-perovskite and hexagonal structures.

Table S1 lists twelve crystal structures of  $\text{BiPbTi}_2\text{O}_6$ , including ten lowest energy structures predicted by CALYPSO, perovskite anti-polar structure with *Pmma* symmetry and post-perovskite anti-polar structure with *Pmmm* symmetry. All the energies in Table S1 are normalized to per formula unit (i.e., 10-atom  $\text{BiPbTi}_2\text{O}_6$ ). The total energy of post-perovskite *Pmm2* structure (the one with the lowest energy) is set as the zero point.

## II. STRUCTURAL INFORMATION OF AVAILABLE SUBSTRATES

TABLE S2. Structural information of perovskite oxide substrates  $\text{KTaO}_3$  and  $\text{NdScO}_3$ , calculated by DFT-PBEsol method. The experimental lattice constants, taken from Ref. [2] are also shown in the parentheses for comparison.

| Substrate        | Cell parameters         | Atom type | Wyckoff site | X     | Y     | Z     |
|------------------|-------------------------|-----------|--------------|-------|-------|-------|
| $\text{KTaO}_3$  | $a = 4.001$ (3.988) Å   |           |              |       |       |       |
|                  | $b = 4.001$ (3.988) Å   | K1        | 1b           | 0.500 | 0.500 | 0.500 |
|                  | $c = 4.001$ (3.988) Å   | Ta1       | 1a           | 0.000 | 0.000 | 0.000 |
|                  | $\alpha = 90.000^\circ$ | O1        | 3d           | 0.500 | 0.000 | 0.000 |
|                  | $\beta = 90.000^\circ$  |           |              |       |       |       |
|                  | $\gamma = 90.000^\circ$ |           |              |       |       |       |
| $\text{NdScO}_3$ | $a = 5.496$ (5.57) Å    |           |              |       |       |       |
|                  | $b = 5.752$ (5.77) Å    | Nd1       | 4c           | 0.250 | 0.482 | 0.437 |
|                  | $c = 7.886$ (7.99) Å    | Sc1       | 4b           | 0.000 | 0.500 | 0.000 |
|                  | $\alpha = 90.000^\circ$ | O1        | 8d           | 0.062 | 0.192 | 0.194 |
|                  | $\beta = 90.000^\circ$  | O2        | 4c           | 0.250 | 0.623 | 0.048 |
|                  | $\gamma = 90.000^\circ$ |           |              |       |       |       |

We study two perovskite oxide substrates  $\text{KTaO}_3$  and  $\text{NdScO}_3$  [2]. As shown in Table S2, the DFT (PBEsol) calculated lattice constants of  $\text{KTaO}_3$  and  $\text{NdScO}_3$  are in good agreement with the experimental lattice constants (within 1% difference). We find that cubic perovskite  $\text{KTaO}_3$  (cubic lattice constant of  $\sim 4.00$  Å) and orthorhombic perovskite  $\text{NdScO}_3$  (pseudo-cubic lattice constant of  $\sim 4.08$  Å) can impose tensile strain sufficiently to stabilize perovskite  $Pmm2$   $\text{BiPbTi}_2\text{O}_6$  in thin film form. In our main text, the heterostructure of  $\text{BiPbTi}_2\text{O}_6/\text{PbTiO}_3$  is simulated to growth on the substrate of  $\text{KTaO}_3$ .

### III. PRESSURE AND STRAIN STUDY INCLUDING $P1$ AND $I4mm$ STRUCTURES

In this section, we study more crystal structures under pressure and strain. We consider not only the three lowest energy structures (post-perovskite  $Pmm2$ , perovskite  $Pmn2_1$  and perovskite  $Pmm2$ ), but also the other two low-energy structures (a non-perovskite  $P1$  and perovskite  $I4mm$ ). Panel **a** of Fig. S1 shows the pressure dependence and panel **b** of Fig. S1 shows the strain dependence. The conclusion in the main text does not change after we consider more low-energy structures.

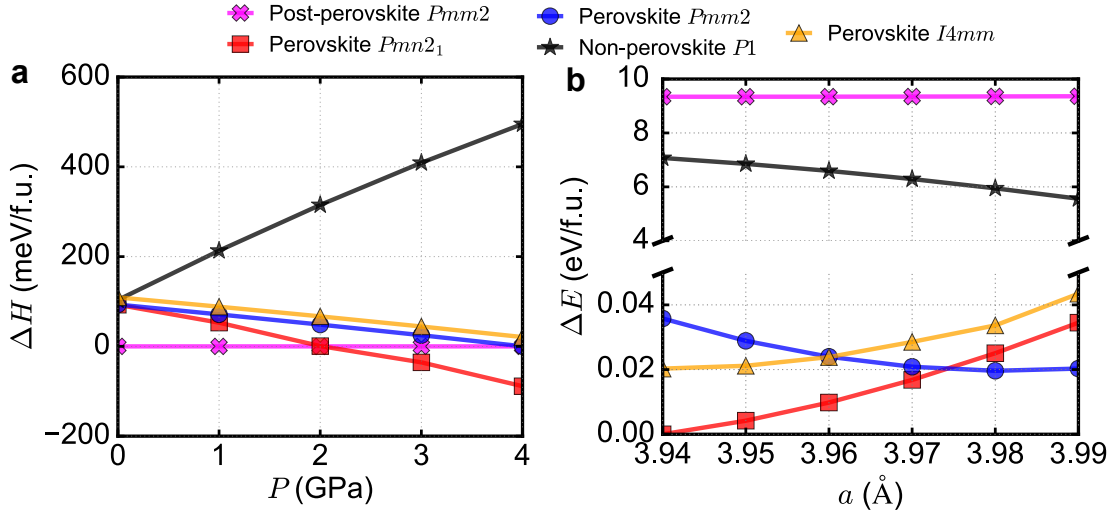

FIG. S1. Pressure and strain study on post-perovskite  $Pmm2$ , perovskite  $Pmn2_1$ , perovskite  $Pmm2$ , non-perovskite  $P1$ , and perovskite  $I4mm$  structures. Panel **a** shows the enthalpy difference  $\Delta H$  as a function of pressure. The enthalpy of post-perovskite  $Pmm2$  structure under each pressure is set as zero point.  $\Delta E$  has the unit of meV/f.u.. Panel **b** shows the energy difference  $\Delta E$  as a function of epitaxial strain. The energy of perovskite  $Pmn2_1$  with in-plane lattice constant of 3.94 Å is set as zero point. Note that we use a broken  $y$ -axis for  $\Delta E$ . In the top half  $y$ -axis, the energy runs from 4 to 10 eV/f.u.; in the bottom  $y$ -axis, the energy ranges from 0 to 0.04 eV/f.u.. The magenta, red, blue, black, and orange curves correspond to post-perovskite  $Pmm2$ , perovskite  $Pmn2_1$ , perovskite  $Pmm2$ , non-perovskite  $P1$ , and perovskite  $I4mm$  structures, respectively.

#### IV. THE DOS OF POST-PEROVSKITE $Pmm2$ STRUCTURE

In this section, Fig. S2 shows the total density of states (DOS) and orbital projected densities of states of post-perovskite  $Pmm2$   $\text{BiPbTi}_2\text{O}_6$ . The DOS at the Fermi level is mainly composed of O-2p, Bi-6p and Pb-6p states, with very small contributions from Ti-3d, Bi-6s and Pb-6s states.

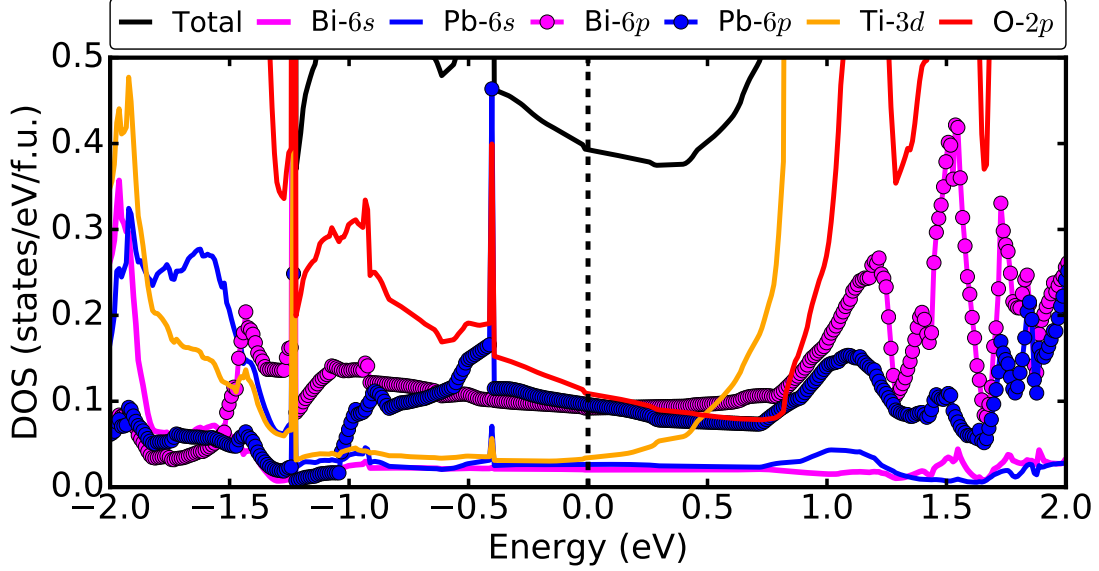

FIG. S2. Total density of states (black curve) and projected densities of states onto Bi-6s (magenta curve), Bi-6p (magenta curve with circle markers), Pb-6s (blue curve), Pb-6p (blue curve with circle markers), Ti-3d (orange curve) and O-2p orbitals (red curve). The Fermi level (the vertical dashed line) is set to zero energy.



## V. PbTiO<sub>3</sub> UNDER BI-AXIAL STRAIN

In experiment, bulk PbTiO<sub>3</sub> displays a spontaneous polarization of about 0.75 C/m<sup>2</sup> at 295 K with  $c/a$  ratio of 1.063 and space group of  $P4mm$  [3, 4]. In this section, we use first-principles calculations (DFT-PBEsol) to study PbTiO<sub>3</sub> under bi-axial strain. In structural optimizations, we use an energy cutoff of 600 eV and  $\mathbf{k}$  mesh of  $17 \times 17 \times 17$ . The convergence thresholds of energy and atomic Hellmann-Feynman forces are  $10^{-9}$  eV and  $10^{-4}$  eV/Å, respectively. We fix the in-plane epitaxial lattice constants ( $a_x = a_y = a$ ) and allow the out-of-plane lattice constant  $a_z = c$  to change. All the internal atomic coordinates are fully relaxed. We study two different polarization orientations: if the polarization is along  $z$ -axis, the state is referred to as “out-of-plane polarization”; if the polarization is either along  $x$ -axis or  $y$ -axis, the state is referred to as “in-plane polarization”.

We change the in-plane epitaxial lattice constant  $a$  and study the energy difference between the “out-of-plane polarization” and the “in-plane polarization” states as a function of  $a$ . The results are shown in Fig. S3a. There is a critical lattice constant  $a_c \simeq 3.97$  Å at which the two states are degenerate. If the epitaxial lattice constant is less than  $a_c$ , the “out-of-plane polarization” state is more energetically favorable. If the epitaxial lattice constant exceeds  $a_c$ , the “in-plane polarization” state becomes more stable. Fig. S3b shows the  $c/a$  ratio of both “out-of-plane polarization” and “in-plane polarization” states as a function of the in-plane epitaxial lattice constant  $a$ . We note that without any strain, our calculations find that bulk PbTiO<sub>3</sub> has lattice constants  $a_x = a_y = 3.89$  Å and  $a_z = 4.17$  Å with its polarization pointing along  $z$  axis. This indicates that if we want to stabilize an in-plane polarization in PbTiO<sub>3</sub> thin films, we need at least 2% bi-axial tensile strain.

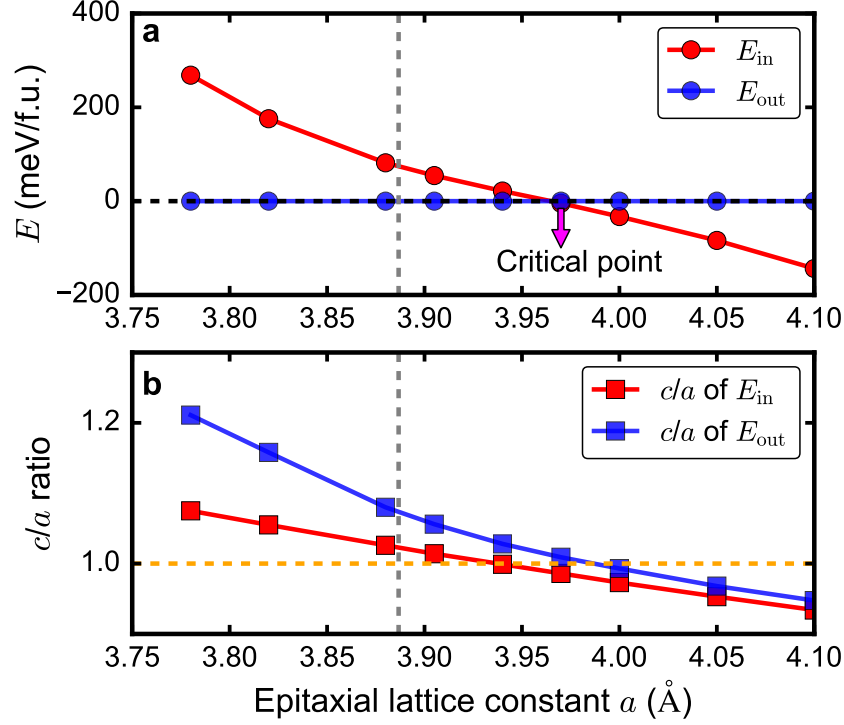

FIG. S3. PbTiO<sub>3</sub> under bi-axial strain. Panel **a**: total energies of “in-plane polarization” state ( $E_{\text{in}}$ ) and “out-of-plane polarization” state ( $E_{\text{out}}$ ) of PbTiO<sub>3</sub> under bi-axial strain. For each given epitaxial lattice constant  $a$ ,  $E_{\text{out}}$  is chosen as the zero energy. At  $a = 3.97$  Å, the two states are degenerate. When  $a < 3.97$  Å, the “out-of-plane polarization” state is more energetically favorable. When  $a > 3.97$  Å, the “in-plane polarization” state is more stable. Panel **b**: the  $c/a$  ratio of both “in-plane polarization” state and “out-of-plane polarization” state as a function of epitaxial lattice constant  $a$ . In both panels, the grey dashed line refers to strain-free PbTiO<sub>3</sub> which has theoretical lattice constants  $a_x = a_y = 3.89$  Å and  $a_z = 4.17$  Å.

## VI. UNIFORM STRAIN IN EPITAXIAL $\text{BiPbTi}_2\text{O}_6$ THIN FILM FROM EXPERIMENTAL PERSPECTIVE

In our DFT calculations, the  $\text{BiPbTi}_2\text{O}_6/\text{PbTiO}_3$  heterostructure is simulated by constraining its in-plane lattice constant to that of  $\text{KTaO}_3$  substrate ( $a = 4.00 \text{ \AA}$ , see Table S2). The entire heterostructure is under *uniform* tensile strain. Under this strain, the  $Pmm2$  perovskite phase is indeed stabilized (see Fig. 4 in the main text). We find the metastable (even unstable and unusual polymorphs) phase can appear via applying uniform epitaxial strains to thin films [5–8]. Such epitaxial stabilization can be understood by the theory of free energy minimization, in which the energy of coherent and semicoherent interfaces is much lower than that of noncoherent ones [9]. Therefore, the formation of low-energy interfaces and the minimization of overall free energy of the system due to the contribution of volume strain energy usually give rise to the experimentally observed metastable and even unstable structures.

Specifically for oxide heterostructures, experimentalists find that the critical thickness below which the entire thin film is under *uniform* strain is typically about 10 nm and sometimes can exceed 100 nm [10]. In our case, the thickness of  $\text{BiPbTi}_2\text{O}_6/\text{PbTiO}_3$  heterostructure (in Fig. 4 in the main text) is only 4 nm, which is far below the critical thickness for uniform strain. Furthermore, in our  $\text{BiPbTi}_2\text{O}_6/\text{PbTiO}_3$  heterostructure,  $\text{PbTiO}_3$  has a polarization parallel to the interface. This means that the depolarization field in  $\text{PbTiO}_3$  thin film can be fully screened by the two electrodes (see the “toy device” in Fig. S4). Therefore the thickness of  $\text{PbTiO}_3$  films can be further reduced without suppressing its polarization. Based on the above reasons, our  $\text{BiPbTi}_2\text{O}_6/\text{PbTiO}_3$  heterostructure is anticipated to be uniformly strained and thus can be stabilized on  $\text{KTaO}_3$  or  $\text{NdScO}_3$  substrate (see Section VIII).

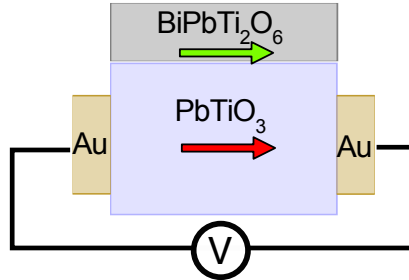

FIG. S4. A model device based on  $\text{BiPbTi}_2\text{O}_6/\text{PbTiO}_3$ . Au only works as electrode.

## VII. DENSITY OF STATES OF $\text{BiPbTiO}_6/\text{PbTiO}_3$ INTERFACE

Total density of states and layer-resolved density of states projected onto Ti-3d orbitals for both parallel and anti-parallel states are shown in Fig. S5. The layer-resolved conduction electrons in the main text are calculated by integrating the partial density states of Ti-3d orbitals.

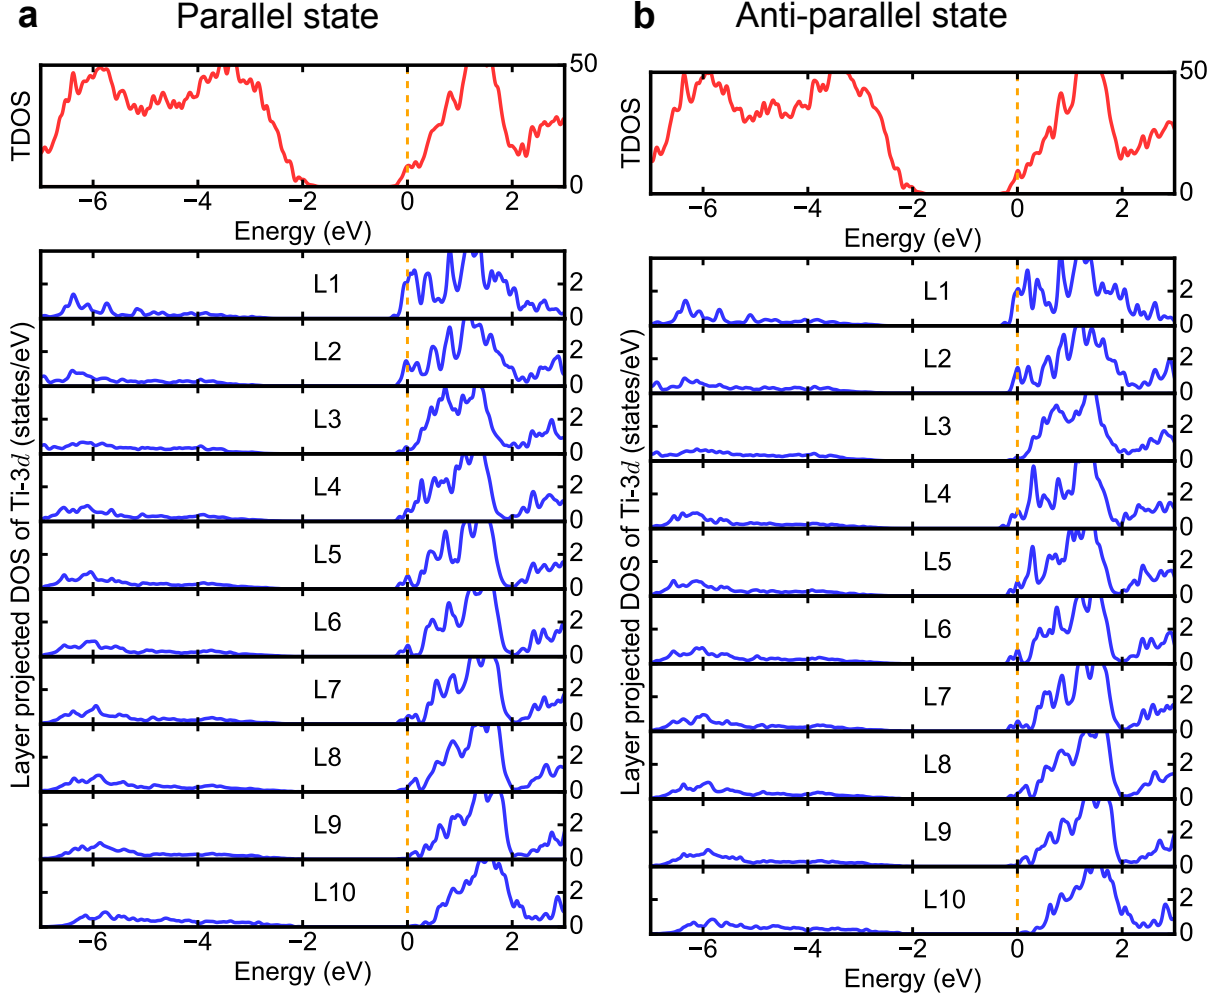

FIG. S5. Total density of states (TDOS) and the layer-resolved density of states projected onto Ti-3d orbitals (layer projected DOS). Panel **a**: parallel state. Panel **b**: anti-parallel state. Red and blue curves correspond to TDOS and layer projected DOS, respectively. L1...L10 refer to the TiO<sub>2</sub> layers of the  $\text{BiPbTiO}_6/\text{PbTiO}_3$  heterostructure (the ordering is consistent with Fig. 5 in the main text). The orange dashed line is Fermi level, which is set to zero energy.

## VIII. THE CHARGE LEAKAGE IN $\text{BiPbTi}_2\text{O}_6$ /FERROELECTRIC HETEROSTRUCTURE

We note that in Fig. 5 of our main text charge leakage into  $\text{PbTiO}_3$  is non-negligible in the  $\text{BiPbTi}_2\text{O}_6/\text{PbTiO}_3$  heterostructure. This charge leakage is due to “proximate effect” that  $\text{PbTiO}_3$  has empty Ti  $d^0$  states while  $\text{BiPbTi}_2\text{O}_6$  has  $0.5e$  in the  $d$  orbitals per Ti site. Charge transfer occurs from the Ti atoms in  $\text{BiPbTi}_2\text{O}_6$  to the Ti atoms in  $\text{PbTiO}_3$  thin films, a phenomenon similar to  $\text{LaTiO}_3/\text{SrTiO}_3$  interface [11, 12]. To prevent charge leakage, we can use  $\text{PbTi}_{1-x}\text{Zr}_x\text{O}_3$  (PZT) to replace  $\text{PbTiO}_3$ . The mechanism is that Zr has  $4d$  orbitals, whose energy is higher than Ti  $3d$  orbitals. To demonstrate that, we replace  $\text{PbTiO}_3$  by  $\text{PbZrO}_3$  in our heterostructure and re-do the calculations. Fig. S6 shows the conduction electrons in Ti- $d$  and Zr- $d$  orbitals. We find that charge leakage is completely suppressed and all the conduction electrons are confined in Ti- $d$  orbitals in  $\text{BiPbTi}_2\text{O}_6$ . A direct simulation of PZT requires a much larger supercell and a proper treatment of random alloying, which is beyond the capability of our computation resources. However, the physics trend is clear: the more Ti atoms are replaced by Zr atoms, the weaker the charge leakage. Usually PZT with  $x \sim 0.2 - 0.5$  is widely used in ferroelectric heterostructures [13–16].

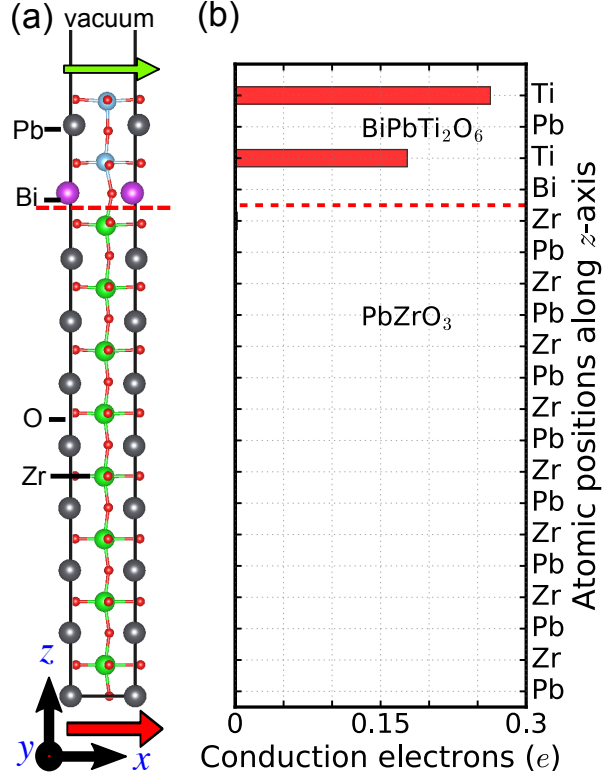

FIG. S6. DFT calculation of BiPbTi<sub>2</sub>O<sub>6</sub>/PbZrO<sub>3</sub> heterostructure. **a** Atomic structure of the BiPbTi<sub>2</sub>O<sub>6</sub>/PbZrO<sub>3</sub> heterostructure: The red (green) arrow refers to PbZrO<sub>3</sub> polarization (BiPbTi<sub>2</sub>O<sub>6</sub> polar displacements). **b** Layer-resolved conduction electrons on Ti and Zr atoms. The red dashed lines indicate the interface between PbZrO<sub>3</sub> and BiPbTi<sub>2</sub>O<sub>6</sub>.

## IX. POLAR DISPLACEMENTS IN THIN FILMS OF POLAR METAL $\text{BiPbTi}_2\text{O}_6$

There is “size effects” in ferroelectric thin films [17]. With the thickness of ferroelectric thin films decreasing, depolarization fields (if not fully screened) reduce and sometimes completely suppress the polarization [18, 19].

However, polar metals do not have such a “size effect” because free electrons in metals fully screen depolarization fields in both bulk and thin films. To support that, we perform two additional calculations.

The first calculation is a thought-experiment. We calculate a free-standing one unit cell  $\text{BiPbTi}_2\text{O}_6$  thin film. We find that down to one unit cell,  $\text{BiPbTi}_2\text{O}_6$  is still polar. The polar displacements of free-standing one unit cell  $\text{BiPbTi}_2\text{O}_6$  thin film are shown in Fig. S7, which are compared to bulk  $\text{BiPbTi}_2\text{O}_6$ . This shows that there is no “size effect” in thin films of polar metal  $\text{BiPbTi}_2\text{O}_6$ .

The second calculation is to study “proximity effect” in  $\text{BiPbTi}_2\text{O}_6$  thin films. Instead of a  $\text{BiPbTi}_2\text{O}_6/\text{PbTiO}_3$  heterostructure, we calculate a  $\text{BiPbTi}_2\text{O}_6/\text{SrTiO}_3$  heterostructure, in which  $\text{SrTiO}_3$  is paraelectric. Fig. S8 shows the optimized structure in our DFT calculations and the corresponding polar displacements along  $x$ -axis. We find that the polar displace-

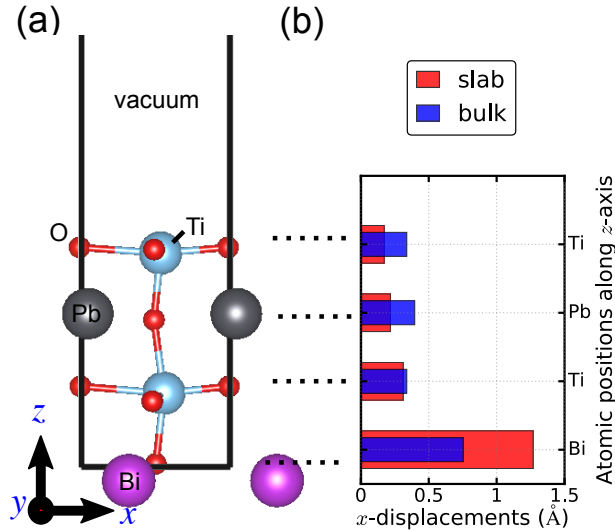

FIG. S7. **a** Optimized structure of a free-standing one unit cell  $\text{BiPbTi}_2\text{O}_6$  thin film. **b** The comparison of layer-resolved polar displacements between one unit cell  $\text{BiPbTi}_2\text{O}_6$  thin film and the bulk phase.

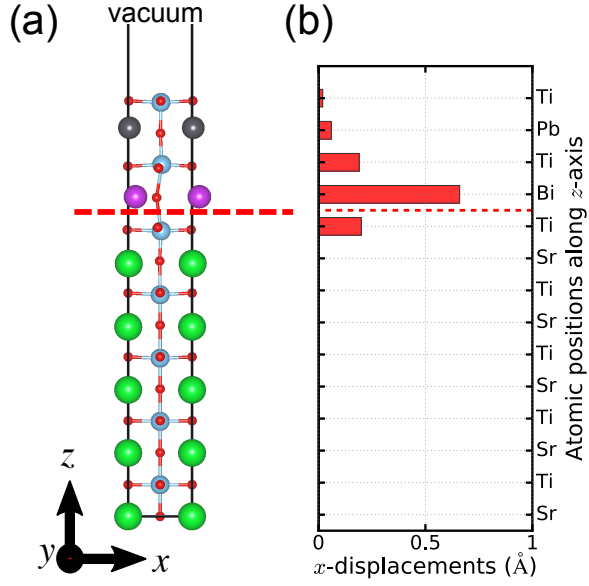

FIG. S8. **a** The optimized structure of BiPbTi<sub>2</sub>O<sub>6</sub>/SrTiO<sub>3</sub> interface. The vacuum layer is about 15 Å in our DFT model. **b** The polar displacements along  $x$ -axis in BiPbTi<sub>2</sub>O<sub>6</sub>/SrTiO<sub>3</sub> interface. The dashed red lines indicate the interface between BiPbTi<sub>2</sub>O<sub>6</sub> and SrTiO<sub>3</sub>.

ments in BiPbTi<sub>2</sub>O<sub>6</sub> still exist. In addition, the structural coupling between BiPbTi<sub>2</sub>O<sub>6</sub> and SrTiO<sub>3</sub> drives the interfacial Ti atom in SrTiO<sub>3</sub> to be polar (see Fig. S8). This indicates that the polar displacements in BiPbTi<sub>2</sub>O<sub>6</sub> thin films are *not* due to proximity coupling with PbTiO<sub>3</sub>. In fact, they are so strong that they can drive a paraelectric material (such as SrTiO<sub>3</sub>) to be polar close to the interface.



## X. SWITCHING OF MULTI-LAYER $\text{BiPbTi}_2\text{O}_6$ FILMS

To support the physical picture of switching multi-layer BPTO in the main text, we perform additional calculations of two-unit-cell BPTO thin films on  $\text{PbTiO}_3$ . Fig. S9 shows different configurations of polar displacements of BPTO and polarization of  $\text{PbTiO}_3$ . The red arrow is the polarization of entire  $\text{PbTiO}_3$  thin film. The green arrow refers to the polar displacements of *each* unit cell of BPTO. Since there are two unit cells of BPTO, then there are altogether four different configurations. Our calculations find that their total energies are  $E_I < E_{II} < E_{III} < E_{IV}$ . This energy order is easy to understand: both the interface and bulk BPTO prefers to have a parallel coupling between polar displacements and polarization. In configuration I, both the polar displacements of BPTO between the two unit cells and the polarization of  $\text{PbTiO}_3$  are parallel, which leads to the lowest total energy. In configuration IV, the polar displacements of  $\text{BiPbTi}_2\text{O}_6$  between the two unit cells are *antiparallel*. The polar displacements of the bottom layer  $\text{BiPbTi}_2\text{O}_6$  is also *antiparallel* to the polarization of  $\text{PbTiO}_3$ . The two antiparallel couplings combined result in the highest total energy. The switching process is as follows: we start from configuration III in which the polarization of  $\text{PbTiO}_3$  is switched by an electric field. The interfacial coupling drives the bottom unit cell of  $\text{BiPbTi}_2\text{O}_6$  to switch its polar displacements (this is configuration II). Then the bulk coupling in  $\text{BiPbTi}_2\text{O}_6$  drives the top unit cell of  $\text{BiPbTi}_2\text{O}_6$  to switch its polar displacements (this is configuration I). This entire process is favored by thermodynamics because the total energy monotonically decreases from configuration III to II and finally to I.

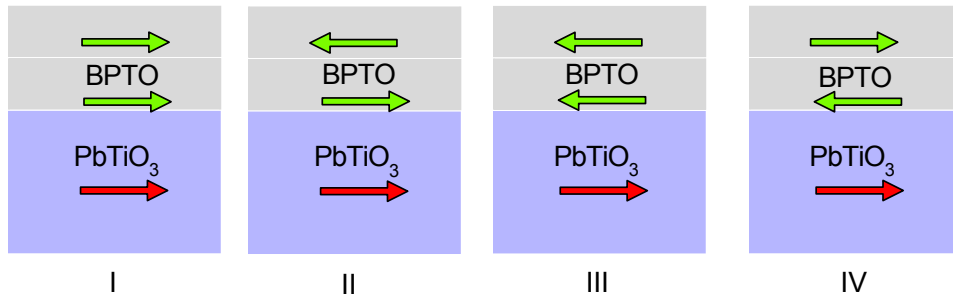

FIG. S9. Four different configuration of the heterostructure composed of  $\text{PbTiO}_3$  thin film and two unit cells of  $\text{BiPbTi}_2\text{O}_6$ . The red arrow refers to the polarization of  $\text{PbTiO}_3$  thin film. The green arrows refer to the polar displacements of *each* unit cell of  $\text{BiPbTi}_2\text{O}_6$ .

- 
- [1] Graham King and Patrick M. Woodward, “Cation ordering in perovskites,” *J. Mater. Chem.* **20**, 5785–5796 (2010).
- [2] Abhijit Biswas, Chan-Ho Yang, Ramamoorthy Ramesh, and Yoon H. Jeong, “Atomically flat single terminated oxide substrate surfaces,” *Prog. Surf. Sci.* **92**, 117–141 (2017).
- [3] W. Zhong, R. D. King-Smith, and David Vanderbilt, “Giant LO-TO splittings in perovskite ferroelectrics,” *Phys. Rev. Lett.* **72**, 3618–3621 (1994).
- [4] M. Dawber, C. Lichtensteiger, M. Cantoni, M. Veithen, P. Ghosez, K. Johnston, K. M. Rabe, and J.-M. Triscone, “Unusual behavior of the ferroelectric polarization in  $\text{PbTiO}_3/\text{SrTiO}_3$  superlattices,” *Phys. Rev. Lett.* **95**, 177601 (2005).
- [5] A Trampert, O Brandt, H Yang, and KH Ploog, “Direct observation of the initial nucleation and epitaxial growth of metastable cubic GaN on (001) GaAs,” *App. Phys. Lett.* **70**, 583–585 (1997).
- [6] Yaobin Xu, Ji-Hyeon Park, Zhenpeng Yao, Chris Wolverton, Manijeh Razeghi, Jinsong Wu, and Vinayak P. Dravid, “Strain-induced metastable phase stabilization in  $\text{Ga}_2\text{O}_3$  thin films,” *ACS Appl. Mater. Interfaces* **11**, 5536–5543 (2019).
- [7] Anoop R. Damodaran, Sungki Lee, J. Karthik, Scott MacLaren, and Lane W. Martin, “Temperature and thickness evolution and epitaxial breakdown in highly strained  $\text{BiFeO}_3$  thin films,” *Phys. Rev. B* **85**, 024113 (2012).
- [8] D. Sando, Bin Xu, L. Bellaiche, and V. Nagarajan, “A multiferroic on the brink: Uncovering the nuances of strain-induced transitions in  $\text{BiFeO}_3$ ,” *Appl. Phys. Rev.* **3**, 011106 (2016).
- [9] O. Yu. Gorbenko, S. V. Samoilenov, I. E. Graboy, and A. R. Kaul, “Epitaxial stabilization of oxides in thin films,” *Chem. Mater.* **14**, 4026–4043 (2002).
- [10] Tianqi Wang, Koustav Ganguly, Patrick Marshall, Peng Xu, and Bharat Jalan, “Critical thickness and strain relaxation in molecular beam epitaxy-grown  $\text{SrTiO}_3$  films,” *Applied Physics Letters* **103**, 212904 (2013).
- [11] A Ohtomo, D. A. Muller, J. L. Grazul, and HY Hwang, “Artificial charge-modulation in atomic-scale perovskite titanate superlattices,” *Nature* **419**, 378 (2002).
- [12] Okamoto S. and Millis A.J., “Electronic reconstruction at an interface between a mott insulator and a band insulator,” *Nature* **428**, 630 (2004).

- [13] Yi Zhang, Lin Xie, Jeongwoo Kim, Alex Stern, Hui Wang, Kui Zhang, Xingxu Yan, Linze Li, Henry Liu, Gejian Zhao, Hang Chi, Chaitanya Gadre, Qiyin Lin, Yichun Zhou, Ctirad Uher, Tingyong Chen, Ying-Hao Chu, Jing Xia, Ruqian Wu, and Xiaoqing Pan, “Discovery of a magnetic conductive interface in  $\text{PbZr}_{0.2}\text{Ti}_{0.8}\text{O}_3/\text{SrTiO}_3$  heterostructures,” *Nat. Commun.* **9**, 685 (2018).
- [14] Jinsik Choi, Jin-Soo Kim, Inrok Hwang, Sahwan Hong, Ik-Su Byun, Seung-Woong Lee, Sung-Oong Kang, and Bae Ho Park, “Different nonvolatile memory effects in epitaxial  $\text{Pt}/\text{PbZr}_{0.3}\text{Ti}_{0.7}\text{O}_3/\text{LSCO}$  heterostructures,” *Appl. Phys. Lett.* **96**, 262113 (2010).
- [15] Ludwig Feigl, I. B. Misirlioglu, Ionela Vrejoiu, Marin Alexe, and Dietrich Hesse, “Impact of misfit relaxation and a-domain formation on the electrical properties of tetragonal  $\text{PbZr}_{0.4}\text{Ti}_{0.6}\text{O}_3/\text{PbZr}_{0.2}\text{Ti}_{0.8}\text{O}_3$  thin film heterostructures: Experiment and theoretical approach,” *J. Appl. Phys.* **105**, 061607 (2009).
- [16] G. S. Wang, X. J. Meng, J. L. Sun, Z. Q. Lai, J. Yu, S. L. Guo, J. G. Cheng, J. Tang, and J. H. Chu, “ $\text{PbZr}_{0.5}\text{Ti}_{0.5}\text{O}_3/\text{La}_{0.5}\text{Sr}_{0.5}\text{CoO}_3$  heterostructures prepared by chemical solution routes on silicon with no fatigue polarization,” *Appl. Phys. Lett.* **79**, 3476–3478 (2001).
- [17] Shaoping Li, Jeffery A. Eastman, James M. Vetrone, Christopher M. Foster, Robert E. Newnham, and L. Eric Cross, “Dimension and size effects in ferroelectrics,” *Jpn. J. Appl. Phys.* **36**, 5169–5174 (1997).
- [18] I P° Batra and BD Silverman, “Thermodynamic stability of thin ferroelectric films,” *Solid State Commun.* **11**, 291–294 (1972).
- [19] Javier Junquera and Philippe Ghosez, “Critical thickness for ferroelectricity in perovskite ultrathin films,” *Nature* **422**, 506 (2003).
